# Supplementary material for: Entity-aware Transformers for Entity Search
Source: arXiv:2205.00820 source file (2022-05-02)
Supplement: Supplementary file 1 [file Appendix.tex]

\section{appendix}

\begin{table}[h]
	\caption{Legend for queries used in Figures \ref{fig:umap:ent} and \ref{fig:umap:wp}}
	\label{tab:3Queries}
	\begin{tabular}{  p{0.50\columnwidth}}
		
		\textbf{Query}  \\
		\includegraphics{figures/c1.png}\  vietnam war facts \\
		\includegraphics{figures/c2.png}\  south korean girl groups \\
		\includegraphics{figures/c3.png}\  roman architecture  \\
		\includegraphics{figures/c4.png}\  D-Day normandy invasion \\
		\includegraphics{figures/c5.png}\  Indian food \\
		\includegraphics{figures/c6.png}\  german female politicians \\
		\includegraphics{figures/c7.png}\  Give me all companies in Munich \\
		\includegraphics{figures/c8.png}\  Which bridges are of the same type as the Manhattan Bridge? \\

	\end{tabular}
\end{table}
